# Supplementary material for: Length-dependent residence time of contacts in simple polymeric models
Source: arXiv:2412.13563 source file (2024-12-18)
Supplement: Supplementary file 1 [file supp-mat-new.pdf]

## Supplementary Materials

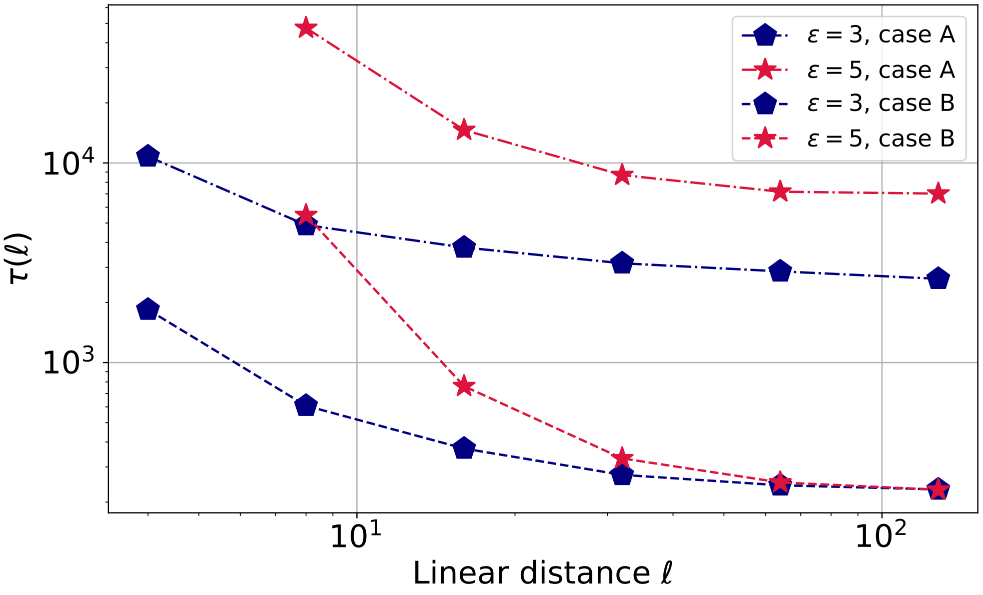


FIG. S1. The mean residence time $\overline{\tau}$ calculated with the two different initial conditions for the ideal chain and for the chain with attracting ends.

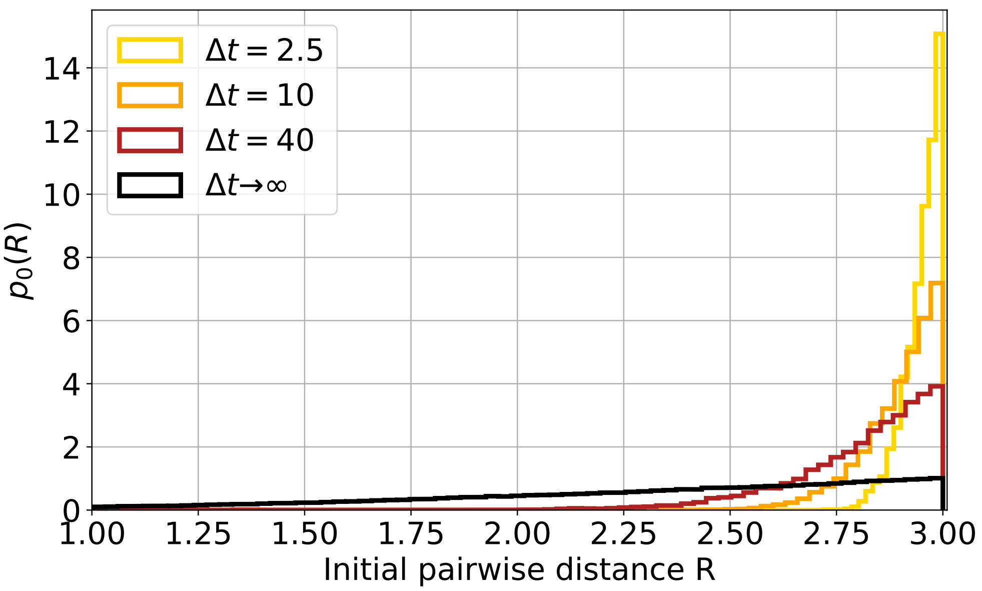


FIG. S2. Examples of the distribution of the initial pairwise distances in case B for different values of the time resolution $\Delta t$. The case $\Delta t \to \infty$ corresponds to case A.

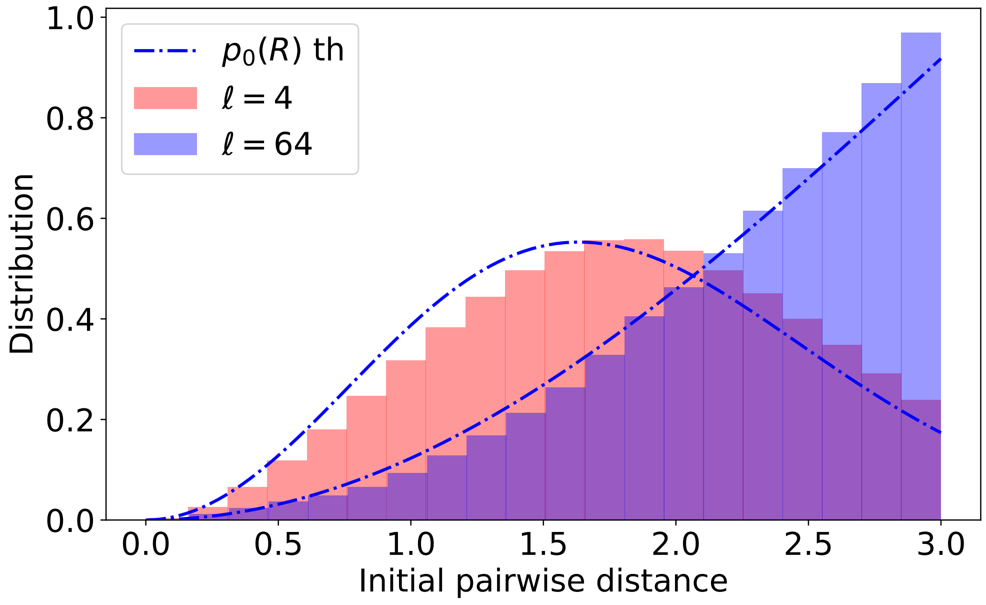


FIG. S3. The distribution of the initial pairwise distance during a contact, for $\ell = 4$ and 64, with initial condition A. The blue dot-dashed line is distribution as predicted by Eq. (B1).

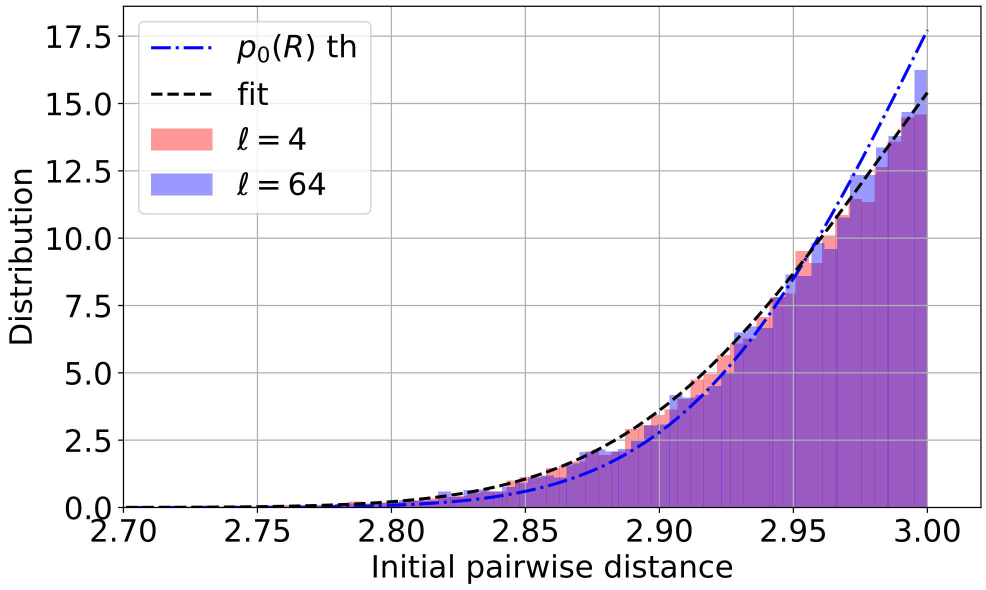


FIG. S4. The distribution of the initial pairwise distance during a contact, for $\ell = 4$ and 64, with initial condition B. The blue dot-dashed line is the approximated distribution as predicted by Eq. (9), while the black dashed line is the fit with a function of the form $p_0(R) = a\,\mathrm{erfc}(\frac{b-R}{c})$.

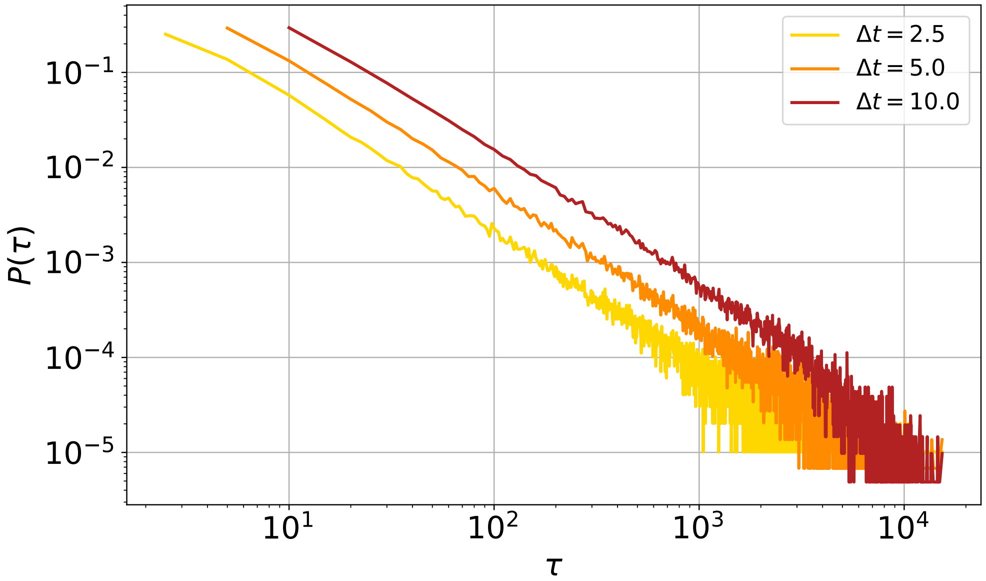


FIG. S5. Examples of the distribution of residence times for $\ell = 8$ and $\epsilon = 3$ computed with three different time resolutions $\Delta t = 2.5$, 5, and 10.

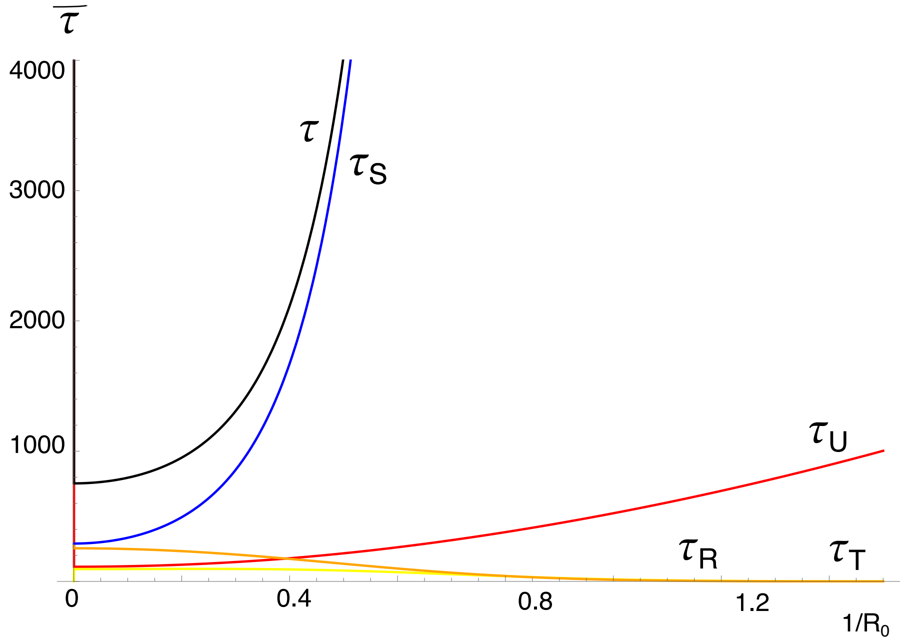


FIG. S6. The function $\overline{\tau}$ as predicted from Eq. (B18) for a polymer with attracting ends and initial conditions of type A, with parameters $\epsilon = 3$, $D = 10^{-3}$, $\beta E_w = 2$ (black curve). The independent variable is $1/R_0$, to better visualize the behaviour at large $R_0$. The colored lines are its four components $\tau_R$, $\tau_S$, $\tau_T$ and $\tau_U$.

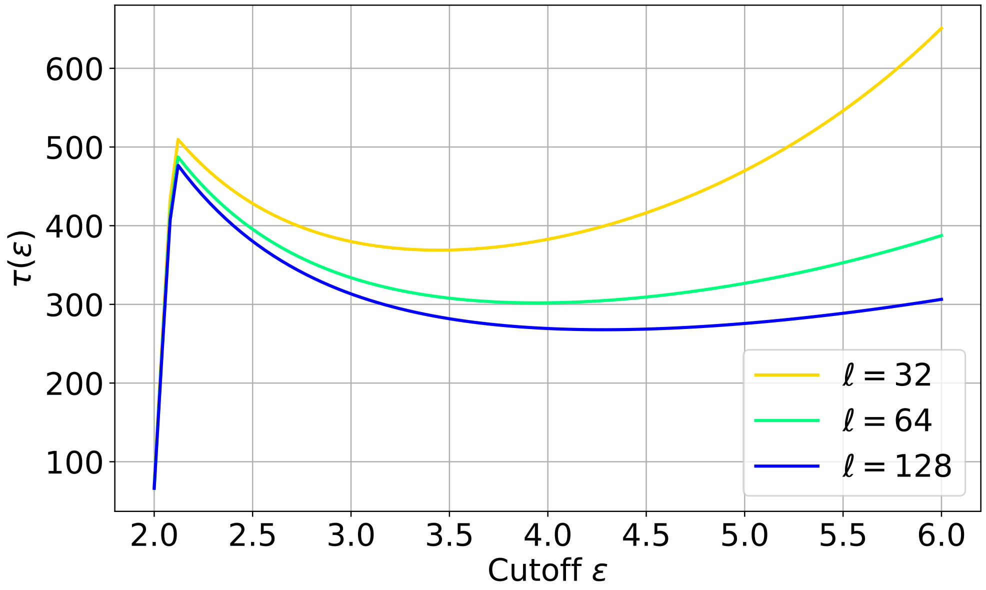


FIG. S7. Residence time of contacts in the ideal chain with a potential well as a function of the contact cutoff, as predicted by Eqs. (D6) and (D7), evaluated at $R = \epsilon - \Delta R$, with $\Delta R = \sqrt{4D\delta t}$, for different values of the genomic distance $\ell$. Thanks to the non-monotonic behaviour of the curves, there are cases where the contact residence time is the same for different values of the cutoff.

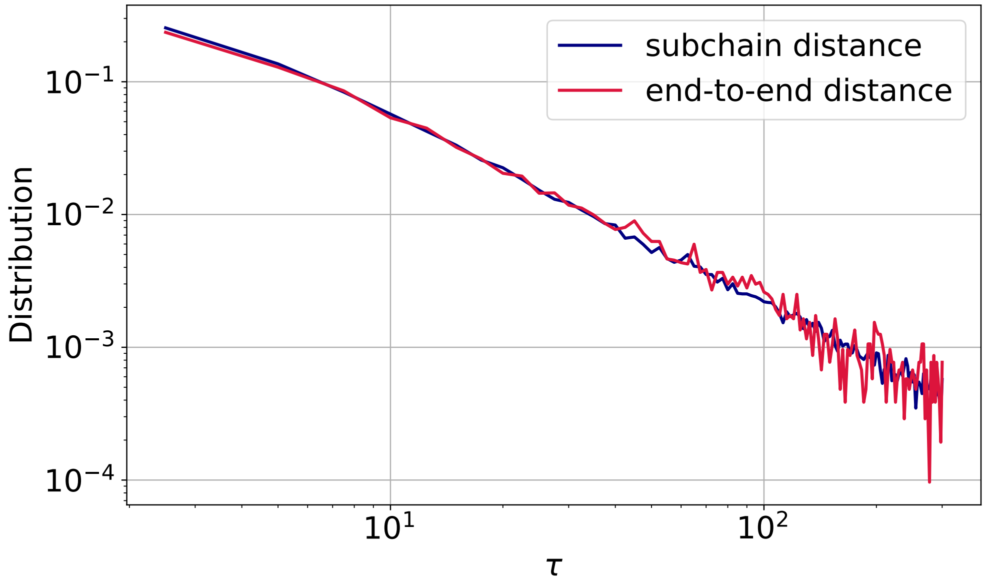


FIG. S8. The distribution of residence times for $\ell = 10$ calculated from simulations of polymers of length $\ell$ and studying pairs of monomers with linear distance $\ell$ in a chain of $N = 1000$ monomer.

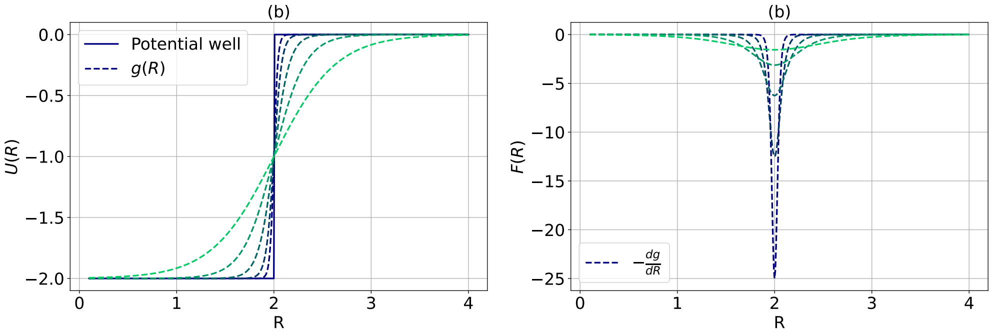


FIG. S9. Approximation of a spherical well by a sigmoid function described by Eq. (A2). A darker colour of the dashed lines corresponds to smaller width parameter $a$. In panel (b) examples of the corresponding forces are plotted for the same values of $a$.

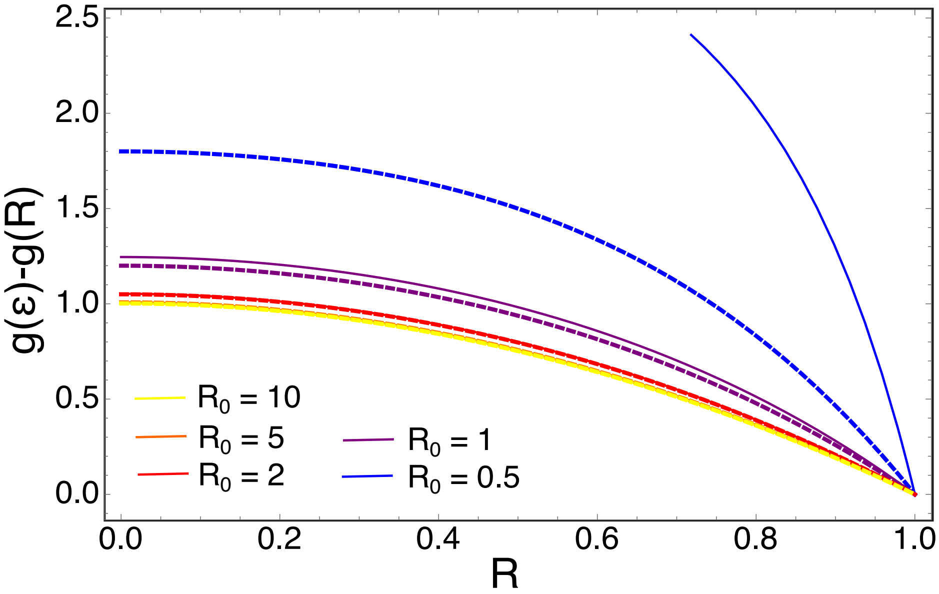


FIG. S10. The values of $g(\epsilon) - g(R)$ in the integral of Eq. (C2) (solid lines), where $g(R) \equiv R^2\,{}_2F_2(R^2/R_0^2)$, are compared with the approximation $\epsilon^2(1 + \epsilon^2/5R_0^2) - R^2(1 + R^2/5R_0^2)$ (dashed lines), for different values of $R_0$ and setting $\epsilon = 1$.

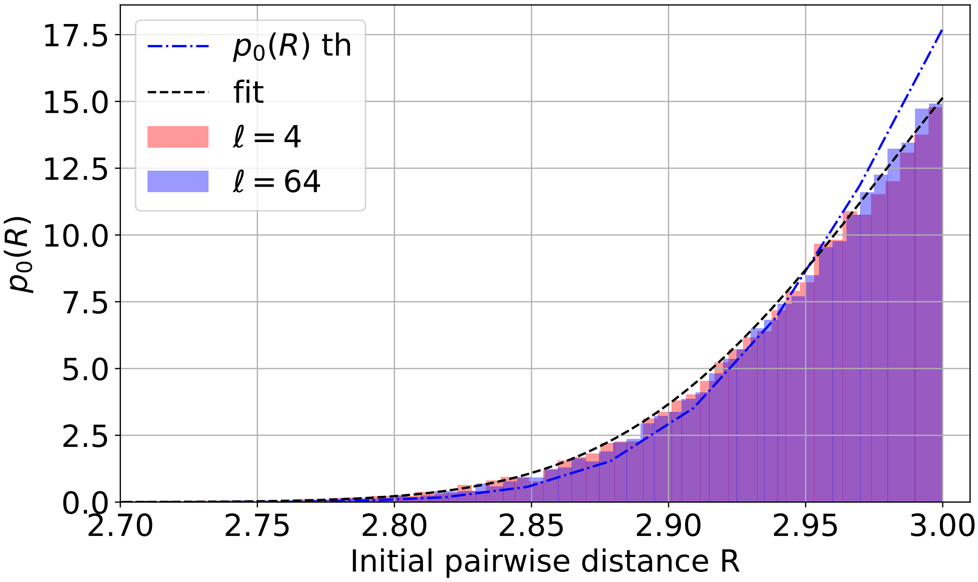


FIG. S11. The distribution of initial distances $p_0(R)$ with contact cutoff $\epsilon = 3$, for small and high $\ell$ (initial condition B), in simulations of an ideal chain with the ends interacting by a potential well. The blue dot-dashed line is the approximated distribution as predicted by Eq. (9), while the black dashed line is the fit with a function of the form $p_0(R) = a\,\mathrm{erfc}(\frac{b-R}{c})$.

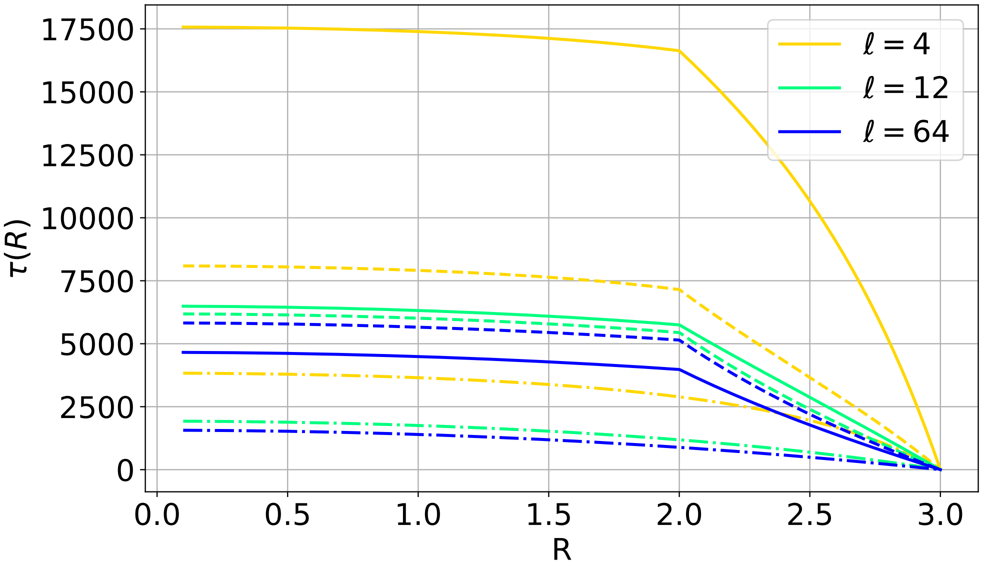


FIG. S12. Examples of the contact residence time as a function of starting distance $R$, as predicted by Eqs. (B6) and (B7) for different values of $\ell$. The parameters used are $\beta E_w = 2$, $R_p = 2$ and $\epsilon = 3$. The dashed lines are the approximated curves predicted by Eq. (13) in the limit $R_0 \to \infty$, while the dashed-dotted lines are the corresponding curves in the absence of a potential well.

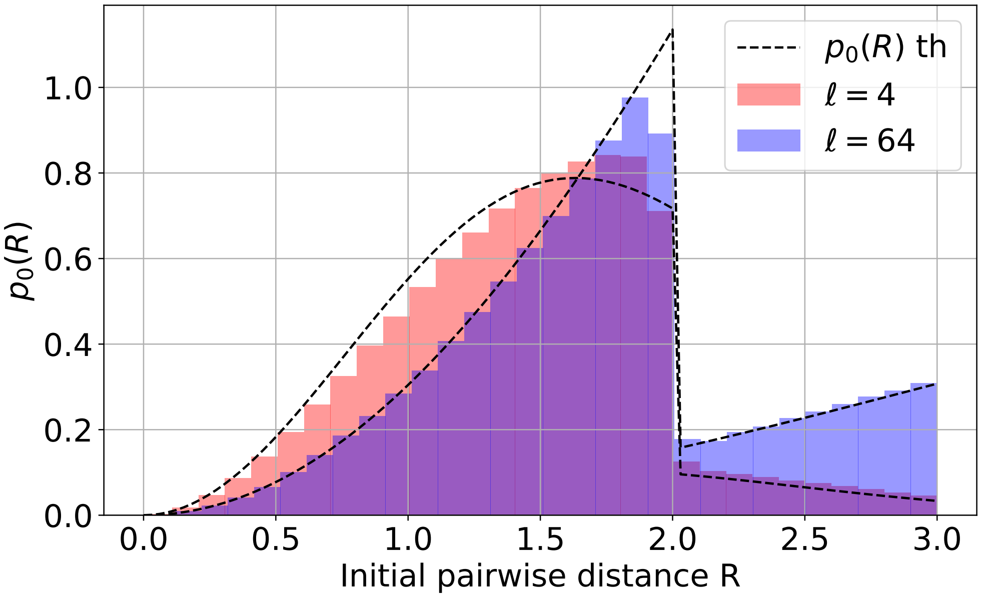


FIG. S13. The distribution of initial distances $p_0(R)$ with contact cutoff $\epsilon = 3$, for small and high $\ell$ (initial condition A), in simulations of an ideal chain with the ends interacting by a potential well.
